# Supplementary material for: A Framework to Learn with Interpretation
Source: arXiv:2010.09345 source file (2022-02-23)

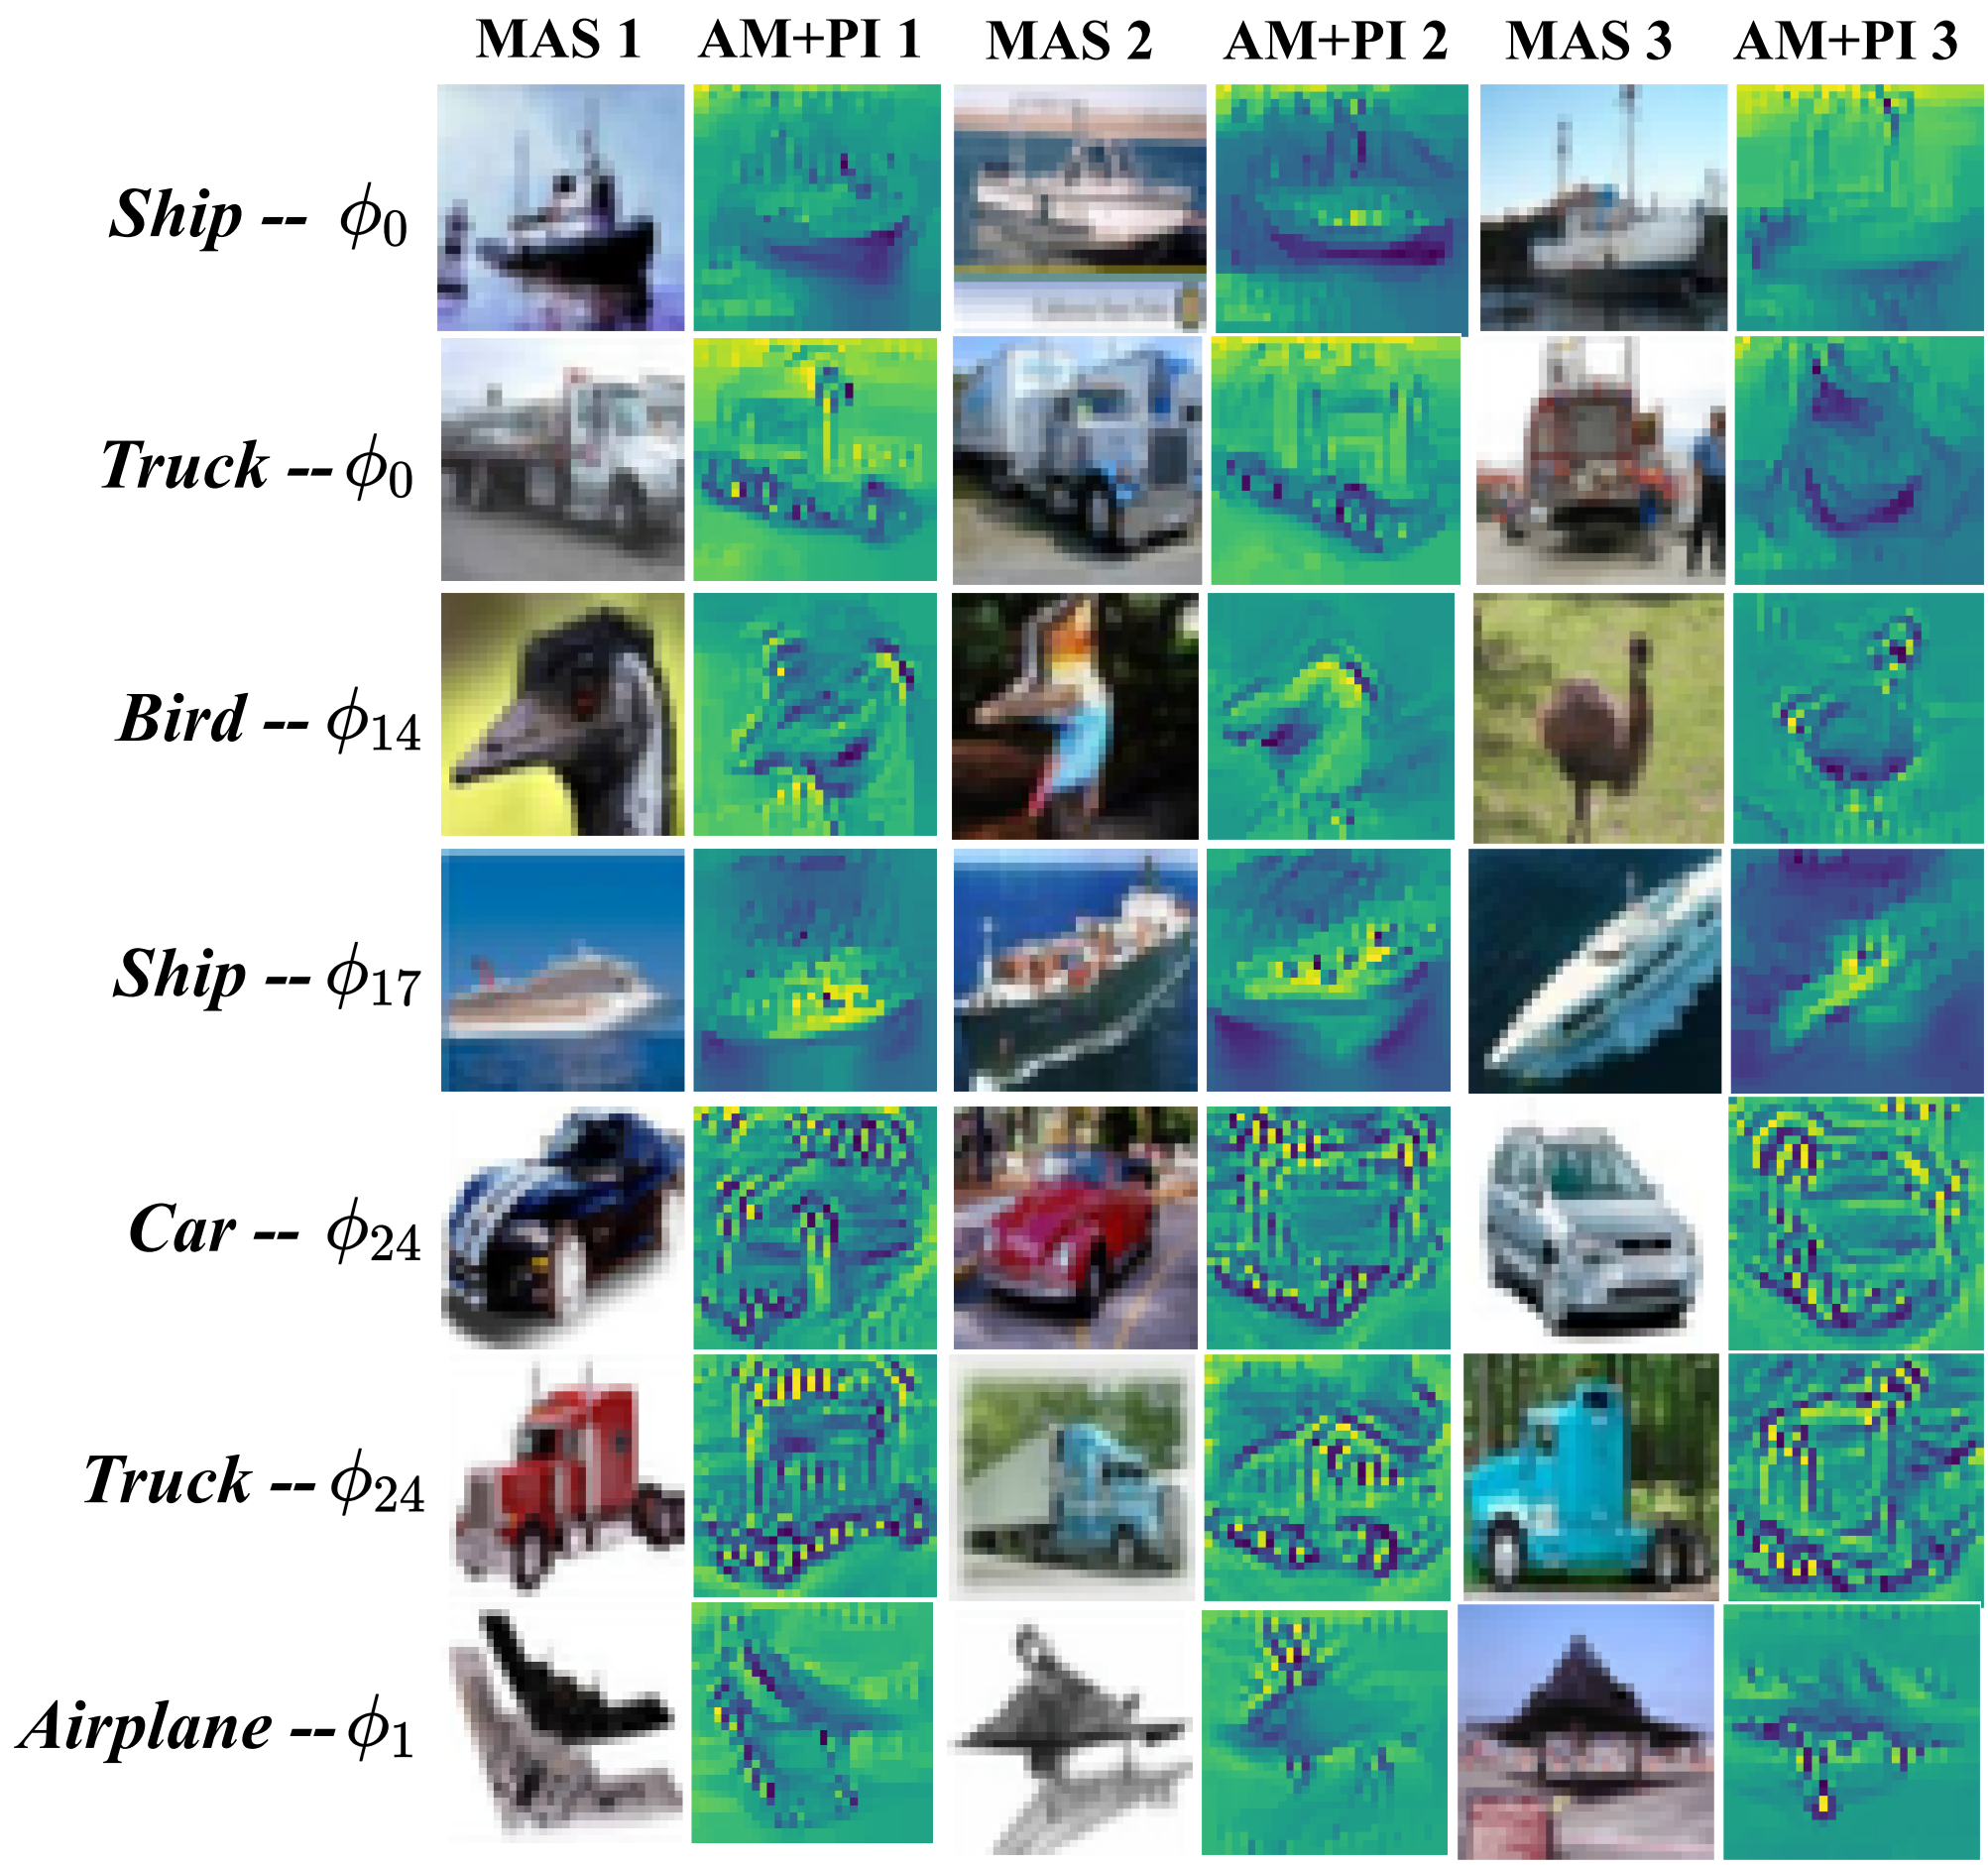

Supplement: Supplementary file 2 [file cifar10_global_viz_ph_v2.pdf]
